# Supplementary material for: What Factors Should Paper-Reviewer Assignments Rely On? Community Perspectives on Issues and Ideals in Conference Peer-Review
Source: arXiv:2205.01005 source file (2022-05-03)
Supplement: Supplementary file 1 [file appendix_suggestions.tex]

\label{app:freeform-suggestions}

TODO add comments
